# Supplementary material for: Dynamic Visual Reasoning by Learning Differentiable Physics Models from Video and Language
Source: arXiv:2110.15358 source file (2021-10-28)
Supplement: Supplementary file 1 [file neural_op_tab.tex]

\begin{table}[htbp]
\centering
\resizebox{1\linewidth}{!}{
\begin{tabular}{cll}
\toprule
Type    & Operation/ Signature & Implementation\\ %Semantics  \\
\midrule
\multirow{10}{2cm}{Input Modules} 
               & \texttt{Objects}  &  $\textit{objects}=\textbf{1}$  \\  
               & $()\rightarrow~\textit{objects}$ \\
               & \texttt{Events}   &  $\textit{events}^{type}$ for $type \in \{in, out, col.\}$ \\
               &  $()\rightarrow ~\textit{events}$ \\
               & \texttt{UnseenEvents}   &   $\textit{events}^{col'}$ and $\textit{events}^{out'}$\\
               &  $()\rightarrow  \textit{events}$  \\
               %& \texttt{AllEvents}  &$()\rightarrow \textit{events}$  &  \\
               %& Returns all possible events on / between any objects & \\
               & \texttt{Start}  &  $M_t=1$ if $t<5$ else $M_t=0$ \\
               & $()\rightarrow  \textit{M}$ \\ 
               & \texttt{end}  &  $M_t=1$ if $t>(T-5)$ else $M_t=0$ \\
                & $()\rightarrow  \textit{M}$ \\
\midrule
\multirow{4}{1cm}{Object Filter Modules} 
& \texttt{Filter\_static\_concept}  & $\min(objs, \text{ObjFilter(\textit{sa})})$ \\
& $ (\text{objs:}~\textit{objects},~\text{sa:}~\textit{concept}) \rightarrow \textit{objects} $ \\
%& \texttt{Filter\_material} & $ (\textit{objects}, \textit{material}) \rightarrow \textit{objects} $  \\
%&  Selects objects from the input list with the input material & \\ 
%& \texttt{Filter\_shape} & $ (\textit{objects}, \textit{shape}) \rightarrow \textit{objects} $  \\
%&  Selects objects from the input list with the input shape & \\
& \texttt{Filter\_dynamic\_concept} & $\min(objects, \text{ObjFilter(\textit{da},t)})$\\
& $ (\text{objs:}~\textit{objects},\text{da:}~\textit{concept},\text{t:}~\textit{frame}) \rightarrow \textit{objects} $ \\
%&  Selects objects in the input frame with the dynamic concept & \\ 
%& \texttt{Filter\_stationary} & $ (\textit{objects}, \textit{frame}) \rightarrow \textit{objects} $  \\
%&  Selects all stationary objects in the input frame & \\
\midrule
\multirow{18}{1cm}{Event Filter Modules} 
& \texttt{Filter\_in} & $\min(objs, \text{events}^{in})$ \\
& $(\text{events}^{in}: \textit{events}, \text{objs:}~\textit{objects}) \rightarrow \textit{events}$ \\
& \texttt{Filter\_out} & $\min(objs, \text{events}^{out})$ \\
& $ (\text{events}^{out}:~\textit{events},\text{objs:}~\textit{objects}) \rightarrow \textit{events} $ \\
& \texttt{Filter\_collision} & $\min(objs^{exp}, \textit{events}^{col.})$  \\
& $ (\text{events}^{col}\text{:}~\textit{events}, \text{objs:}~\textit{objects}) \rightarrow \textit{events} $ \\
& \texttt{Get\_col\_partner} & $\max_{k\in[1,K]}(\text{events}^{col}_{n,k})$  \\
& $ (\text{events}^{col}: \textit{events}, obj_n:~\textit{object} ) \rightarrow \textit{objects}$ \\
& \texttt{Filter\_before}   & $events_n^{in}=-1$ if $t^{in}_n>t^{event1}$ \\
& $(events_n^{in}:~\textit{events}, \text{event1:}~\textit{event})$ \\
& \texttt{Filter\_after} & $events_n^{in}=-1$ if $t^{in}_n<t^{event1}$ \\
& $ (events_n^{in}:~\textit{events}, \text{event1:}~\textit{event}) \rightarrow \textit{events} $  \\
& \texttt{Filter\_order} &  $events_n^{in}>0$ if $order^{in}_n=or$ \\
& $ (events_n^{in}:~\textit{events}, \text{or:}~\textit{order}) \rightarrow \textit{event} $  \\
& \texttt{Filter\_ancestor} & {$ \{\text{event1}_n>0~\text{and}~\text{events1}_n$} \\
& $ (\text{event1:}~\textit{event}, \text{events1:}~\textit{events}) \rightarrow \textit{events} $ & \text{in the causal graph of} event1\} \\
& \texttt{Get\_frame} &  $t^{event1}$ \\
& $ (\text{event1:}~\textit{event}) \rightarrow \textit{frame} $  \\
%& \texttt{Get\_object} & \\
%& $ (\textit{event}) \rightarrow \textit{object} $  \\
\midrule
\multirow{14}{1cm}{Output Modules}
& \texttt{Query\_Attribute} &  $P^{op}=\frac{ObjFilter(op) \cdot i^{op}_a }{\sum_{op'}{ObjFilter(op') \cdot} i^{op'}_a }$\\
& $ (\text{obj:}~\textit{object}, \text{a:}~\textit{attribute}) \rightarrow \textit{concept}$  \\
%& \texttt{Query\_material} & $ (\textit{object}) \rightarrow \textit{material} $  \\
%& Returns the material of the input objects & \\ 
%& \texttt{Query\_shape} & $ (\textit{object}) \rightarrow \textit{shape} $  \\
%& Returns the shape of the input objects & \\ 
& \texttt{Count} & $\sum_n({\text{objs}_n}>0)$ \\
& $ (\text{objs:}~\textit{objects}) \rightarrow \textit{int} $  \\
& \texttt{Exist} & $(\sum_n({\text{objs}_n}>0))>0 $ \\
& $ (\text{objs:}~\textit{objects}) \rightarrow \textit{bool} $  \\
& \texttt{Belong\_to} & $ \text{True if event1} \in \text{events1 else False} $ \\
& $ (\text{event1:}~\textit{event}, \text{events1:}~\textit{events}) \rightarrow \textit{bool} $  \\
& \texttt{Negate} & False if bl else True \\
& $ (\text{bl:}~\textit{bool}) \rightarrow \textit{bool} $  \\
%\midrule
%& \texttt{Unique} & $argmax(objs)$ \\
%&$ (\text{objs:}~\textit{objects}) \rightarrow \textit{object} $    \\
\bottomrule
\end{tabular}
}
\caption{Neural operations in \alias. $\textit{events}^{col'}$ denotes the \textit{collision} events happening at the unseen future frames. $\textit{objs}^{exp} \in \mathbb{R}^{N \times N \times K}$ and $\textit{objs}^{exp}_{n_1, n_2, k}=\max(objs_{n_1}, objs_{n_2})$. $events_{n, k}^{col}$ denotes all the collision events that the $n$-th object get involved at the $k$-th frame.}
\label{tb:neural_op}
\end{table}
