# Supplementary material for: Dynamic Visual Reasoning by Learning Differentiable Physics Models from Video and Language
Source: arXiv:2110.15358 source file (2021-10-28)
Supplement: Supplementary file 2 [file datatype_tab.tex]

\begin{table}[t]
\centering
%\renewcommand{\arraystretch}{0.9}
%\setlength{\tabcolsep}{0.3em}
%\resizebox{1\linewidth}{!}{
\begin{tabular}{ll}
\toprule
Type     & Semantics \\
\midrule
\textit{object} &   A single object in the video. \\
\textit{objects}   & A set of objects in the video. \\
\textit{event}  & A single event in the video. \\
\textit{events}  & A set of events in the video. \\
\textit{order} & The chronological order of an event, \eg ``First'', ``Second'' and ``Last''. \\
%\textit{color}  & An indication of a color, including ``blue'', ``brown'', ``cyan'', ``gray'', ``green'', ``purple'' ,  ``red'' and ``yellow''. \\
%\textit{material} & An indication of a material including ``metal'' and ``rubber''. \\
%\textit{shape} & An indication of a shape including ``cube'', ``cylinder'' and ``sphere''. \\
\textit{static concept} & Object-level static concepts like ``Red'', ``Sphere'' and ``Metal''. \\
\textit{dynamic concept} & Object-level dynamic concepts like ``Moving'' and ``Stationary''. \\
\textit{attribute} & Static attributes including ``Color'', ``Shape'' and ``Material''. \\
\textit{frame}  & The frame number of an event. \\
\textit{int} & A single integer like ``0'' and ``1''. \\
\textit{bool} & A single boolean value, ``True'' or ``False''. \\
\textit{representations} & The visual features that are calculated from object trajectories. \\
\bottomrule
\end{tabular}
\caption{The data types on CLEVRER~\cite{yi2019clevrer}.}
\label{tb:datatype}
\end{table}
